# Supplementary material for: Towards Efficient Modelling of String Dynamics: A Comparison of State Space and Koopman based Deep Learning Methods
Source: arXiv:2408.16650 source file (2024-08-29)
Supplement: Supplementary file 1 [file 07_appendix.tex]

% \section{Appendix: Margin Check}
% This section shows the column margins for the text. \bigskip\newline
